# Supplementary material for: Listening between the Lines: Learning Personal Attributes from Conversations
Source: arXiv:1904.10887 source file (2019-04-24)
Supplement: Supplementary file 1 [file appendix.tex]

\begin{appendices}

\section{Class Distribution}

\begin{table}[h!]
\begin{tabular}{lll}
profession         & MRR   & count \\ \hline
student            & 0.911 & 23    \\
military personnel & 0.799 & 31    \\
scientist          & 0.749 & 19    \\
criminal           & 0.661 & 42    \\
journalist         & 0.611 & 5     \\
astronaut          & 0.565 & 10    \\
monarch            & 0.523 & 4     \\
school teacher     & 0.500 & 2     \\
special agent      & 0.448 & 24    \\
housewife          & 0.406 & 14    \\
child              & 0.379 & 10    \\
detective          & 0.362 & 9     \\
policeman          & 0.341 & 12    \\
musician           & 0.332 & 5     \\
lawyer             & 0.305 & 5     \\
politician         & 0.289 & 4     \\
businessperson     & 0.233 & 15    \\
professor          & 0.186 & 4     \\
nurse              & 0.174 & 3     \\
doctor             & 0.128 & 5     \\
psychologist       & 0.114 & 5     \\
editor             & 0.107 & 3     \\
writer             & 0.096 & 7     \\
engineer           & 0.091 & 1     \\
photographer       & 0.091 & 3     \\
priest             & 0.082 & 4     \\
airplane pilot     & 0.079 & 3     \\
assistant          & 0.071 & 3     \\
actor              & 0.070 & 7     \\
unemployed         & 0.067 & 9     \\
painter            & 0.063 & 2     \\
tv/radio presenter & 0.054 & 2     \\
activist           & 0.046 & 3     \\
explorer           & 0.045 & 3     \\
stewardess         & 0.044 & 2     \\
banker             & 0.043 & 1     \\
waiter             & 0.042 & 1     \\
clerk              & 0.040 & 3     \\
sportsman          & 0.037 & 5     \\
driver             & 0.035 & 4     \\
salesperson        & 0.032 & 3     \\
manager            & 0.028 & 2    
\end{tabular}
\caption{Distribution of MRR and number of occurrences of professions.}
\label{tab3}
\end{table}

\end{appendices}
